# Supplementary material for: Prediction of new sp3 silicon and germanium allotropes from the topology-based multiscale method
Source: arXiv:1701.04667 ancillary file (2017-01-18)
Supplement: Supplementary file 1 [file Supplementary.pdf]

# Prediction of new $sp^3$ silicon and germanium allotropes from the topology-based multiscale method

Vladimir A. Saleev* and Alexandra V. Shipilova†

*Department of Physics, Samara National Research University - Moscow Highway, 34, 443086 Samara, Russia*

Davide M. Proserpio‡

*Università degli Studi di Milano, Dipartimento di Chimica - via Golgi, 19, 20133 Milano, Italy and Samara Center for Theoretical Materials Science (SCTMS), Samara National Research University - Moscow Highway, 34, 443086 Samara, Russia*

Giuseppe Fadda§

*Research and Education Center for Physics of Open Nonequilibrium Systems, Samara National Research University - Moscow Highway, 34, 443086 Samara, Russia*

## Abstract

This article continues our recent publication [I. A. Baburin and D. M. Proserpio and V. A. Saleev and A.V. Shipilova, Phys. Chem. Chem. Phys.17, 1332 (2015)] where we have presented a comprehensive computational study of $sp^3$ carbon allotropes based on the topologies proposed for zeolites. Here we predict six new silicon and six new germanium allotropes which have the same space group symmetries and topologies as those predicted earlier for the carbon allotropes, and study their structural, elastic, vibrational, electronic and optical properties.

PACS numbers: 62.20.-x, 71.20.-b, 78.30.Am, 78.40.Fy

*Electronic address: saleev@samsu.ru
†Electronic address: alexshipilova@samsu.ru
‡Electronic address: davide.proserpio@unimi.it
§Electronic address: gfadda@dmsa.unipd.it

# I. SUPPLEMENTARY MATERIAL

## A. Crystallographic data for the silicon allotropes

Silicon #26: space group $P2/m$ (No. 10); $a = 6.469, b = 3.818, c = 13.27, \beta = 99.61$

| Atomic # | x | y | z |
|---|---|---|---|
| Si1 | 0.340 | 0.500 | 0.942 |
| Si2 | 0.181 | 0.000 | 0.519 |
| Si3 | 0.413 | 0.500 | 0.772 |
| Si4 | 0.325 | 0.500 | 0.458 |
| Si5 | 0.257 | 0.500 | 0.275 |
| Si6 | 0.245 | 0.000 | 0.697 |
| Si7 | 0.121 | 0.000 | 0.943 |
| Si8 | 0.943 | 0.000 | 0.772 |

Silicon #27: space group $C2/m$ (No. 12); $a = 26.415, b = 3.820, c = 6.452, \beta = 94.53$

| Atomic # | x | y | z |
|---|---|---|---|
| Si1 | 0.231 | 0.000 | 0.919 |
| Si2 | 0.887 | 0.500 | 0.950 |
| Si3 | 0.238 | 0.500 | 0.407 |
| Si4 | 0.971 | 0.500 | 0.850 |
| Si5 | 0.029 | 0.000 | 0.371 |
| Si6 | 0.150 | 0.500 | 0.384 |
| Si7 | 0.139 | 0.000 | 0.884 |
| Si8 | 0.884 | 0.000 | 0.473 |

Silicon #28: space group name *Pbam* (No. 55); $a = 11.025, b = 11.661, c = 3.818$

| Atomic # | x | y | z |
|---|---|---|---|
| Si1 | 0.400 | 0.0377 | 0.000 |
| Si2 | 0.376 | 0.150 | 0.500 |
| Si3 | 0.206 | 0.269 | 0.500 |
| Si4 | 0.239 | 0.385 | 0.000 |
| Si5 | 0.012 | 0.195 | 0.500 |
| Si6 | 0.455 | 0.408 | 0.000 |

Silicon #50: space group *Pnma* (No. 62); $a = 11.742, b = 3.826, c = 12.636$

| Atomic # | x | y | z |
|---|---|---|---|
| Si1 | 0.515 | 0.250 | 0.836 |
| Si2 | 0.942 | 0.750 | 0.012 |
| Si3 | 0.661 | 0.250 | 0.963 |
| Si4 | 0.76749 | 0.750 | 0.918 |
| Si5 | 0.908 | 0.750 | 0.634 |
| Si6 | 0.633 | 0.250 | 0.686 |
| Si7 | 0.741 | 0.750 | 0.730 |

Silicon #55: space group name $Pmma$ (No. 51); $a = 13.859, b = 3.827, c = 7.599$

| Atomic # | x | y | z |
|---|---|---|---|
| Si1 | 0.110 | 0.000 | 0.719 |
| Si2 | 0.250 | 0.000 | 0.543 |
| Si3 | 0.662 | 0.000 | 0.985 |
| Si4 | 0.250 | 0.500 | 0.370 |
| Si5 | 0.020 | 0.500 | 0.651 |
| Si6 | 0.619 | 0.500 | 0.824 |

Silicon #88: space group $Pnma$ (No. 62); $a = 19.665, b = 3.837, c = 6.442$

| Atomic # | x | y | z |
|---|---|---|---|
| Si1 | 0.715 | 0.250 | 0.935 |
| Si2 | 0.603 | 0.250 | 0.066 |
| Si3 | 0.789 | 0.250 | 0.21983 |
| Si4 | 0.573 | 0.750 | 0.249 |
| Si5 | 0.545 | 0.250 | 0.750 |
| Si6 | 0.904 | 0.250 | 0.104 |

### B. Crystallographic data for the germanium allotropes

Germanium #26: space group $P2/m$ (No. 10); $a = 6.839, b = 4.056, c = 14.064, \beta =$ 99.48

| Atomic # | x | y | z |
|---|---|---|---|
| Ge1 | 0.339 | 0.500 | 0.941 |
| Ge2 | 0.180 | 0.000 | 0.521 |
| Ge3 | 0.411 | 0.500 | 0.771 |
| Ge4 | 0.324 | 0.500 | 0.459 |
| Ge5 | 0.256 | 0.500 | 0.276 |
| Ge6 | 0.243 | 0.000 | 0.697 |
| Ge7 | 0.121 | 0.000 | 0.942 |
| Ge8 | 0.942 | 0.000 | 0.772 |

Germanium #27: space group $C2/m$ (No. 12); $a$=27.948, $b$=4.054, $c$=6.834, $\beta = 94.519$

| Atomic # | x | y | z |
|---|---|---|---|
| Ge1 | 0.232 | 0.000 | 0.916 |
| Ge2 | 0.887 | 0.500 | 0.949 |
| Ge3 | 0.237 | 0.500 | 0.409 |
| Ge4 | 0.971 | 0.500 | 0.850 |
| Ge5 | 0.030 | 0.000 | 0.371 |
| Ge6 | 0.149 | 0.500 | 0.385 |
| Ge7 | 0.140 | 0.000 | 0.884 |
| Ge8 | 0.884 | 0.000 | 0.474 |

Germanium #28: space group $Pbam$ (No. 55); $a = 11.633, b = 12.349, c = 4.057$

| Atomic # | x | y | z |
|---|---|---|---|
| Ge1 | 0.399 | 0.038 | 0.000 |
| Ge2 | 0.376 | 0.150 | 0.500 |
| Ge3 | 0.207 | 0.270 | 0.500 |
| Ge4 | 0.239 | 0.384 | 0.000 |
| Ge5 | 0.012 | 0.195 | 0.500 |
| Ge6 | 0.456 | 0.408 | 0.00000 |

Germanium #50: space group $Pnma$ (No. 62); $a = 12.410, b = 4.066, c = 13.389$

| Atomic # | x | y | z |
|---|---|---|---|
| Ge1 | 0.514 | 0.250 | 0.838 |
| Ge2 | 0.942 | 0.750 | 0.013 |
| Ge3 | 0.661 | 0.250 | 0.962 |
| Ge4 | 0.766 | 0.750 | 0.918 |
| Ge5 | 0.907 | 0.750 | 0.634 |
| Ge6 | 0.632 | 0.250 | 0.689 |
| Ge7 | 0.741 | 0.750 | 0.732 |

Germanium #55: space group $Pmma$ (No. 51); $a = 14.735, b = 4.057, c = 8.017$

| Atomic # | x | y | z |
|---|---|---|---|
| Ge1 | 0.110 | 0.000 | 0.722 |
| Ge2 | 0.250 | 0.000 | 0.549 |
| Ge3 | 0.663 | 0.000 | 0.983 |
| Ge4 | 0.250 | 0.500 | 0.376 |
| Ge5 | 0.020 | 0.500 | 0.653 |
| Ge6 | 0.622 | 0.500 | 0.820 |

Germanium #88, space group $Pnma$ (No. 62); $a = 20.925, b = 4.067, c = 6.803$

| Atomic # | x | y | z |
|---|---|---|---|
| Ge1 | 0.713 | 0.250 | 0.938 |
| Ge2 | 0.602 | 0.250 | 0.068 |
| Ge3 | 0.790 | 0.250 | 0.221 |
| Ge4 | 0.571 | 0.750 | 0.249 |
| Ge5 | 0.547 | 0.250 | 0.749 |
| Ge6 | 0.904 | 0.250 | 0.103 |

### C. Matrices of the elastic constants $C_{ab}$ for silicon and germanium allotropes

| | Si26 | Si27 | Si28 | Si50 | Si55 | Si88 |
|---|---|---|---|---|---|---|
| $C_{11}$ | 168.705 | 159.176 | 174.359 | 147.247 | 129.351 | 118.139 |
| $C_{22}$ | 164.950 | 164.253 | 146.247 | 162.204 | 169.714 | 160.133 |
| $C_{33}$ | 147.814 | 164.978 | 161.755 | 150.163 | 162.098 | 164.089 |
| $C_{44}$ | 36.594 | 59.471 | 57.656 | 37.482 | 48.232 | 55.576 |
| $C_{55}$ | 45.461 | 45.295 | 39.254 | 44.927 | 47.545 | 50.028 |
| $C_{66}$ | 58.795 | 37.167 | 50.628 | 56.935 | 42.862 | 38.790 |
| $C_{12}$ | 55.120 | 37.425 | 56.104 | 54.962 | 42.331 | 39.377 |
| $C_{13}$ | 47.701 | 47.748 | 37.586 | 57.408 | 57.428 | 50.231 |
| $C_{15}$ | -1.223 | 3.975 | 0 | 0 | 0 | 0 |
| $C_{23}$ | 37.802 | 52.333 | 53.612 | 39.551 | 54.954 | 60.102 |
| $C_{25}$ | 2.334 | -4.084 | 0 | 0 | 0 | 0 |
| $C_{35}$ | 2.794 | -1.331 | 0 | 0 | 0 | 0 |
| $C_{46}$ | 2.794 | -4.068 | 0 | 0 | 0 | 0 |

| | Ge26 | Ge27 | Ge28 | Ge50 | Ge55 | Ge88 |
|---|---|---|---|---|---|---|
| $C_{11}$ | 128.141 | 127.841 | 137.460 | 112.176 | 110.425 | 105.971 |
| $C_{22}$ | 127.878 | 127.900 | 112.423 | 126.344 | 131.293 | 124.455 |
| $C_{33}$ | 122.299 | 126.152 | 126.884 | 121.020 | 124.758 | 122.033 |
| $C_{44}$ | 33.950 | 51.094 | 51.527 | 33.400 | 41.990 | 48.716 |
| $C_{55}$ | 40.889 | 40.961 | 35.201 | 43.506 | 45.317 | 44.455 |
| $C_{66}$ | 51.089 | 34.113 | 46.111 | 50.772 | 39.335 | 35.236 |
| $C_{12}$ | 32.635 | 17.593 | 31.846 | 34.340 | 21.917 | 20.228 |
| $C_{13}$ | 24.510 | 24.624 | 15.396 | 33.947 | 32.794 | 27.435 |
| $C_{15}$ | -1.125 | 3.537 | 0 | 0 | 0 | 0 |
| $C_{23}$ | 18.311 | 31.625 | 33.434 | 17.779 | 30.786 | 36.548 |
| $C_{25}$ | 2.428 | -3.410 | 0 | 0 | 0 | 0 |
| $C_{35}$ | -1.981 | -0.543 | 0 | 0 | 0 | 0 |
| $C_{46}$ | 2.437 | -3.119 | 0 | 0 | 0 | 0 |

## D. Phonon band structure for silicon and germanium allotropes

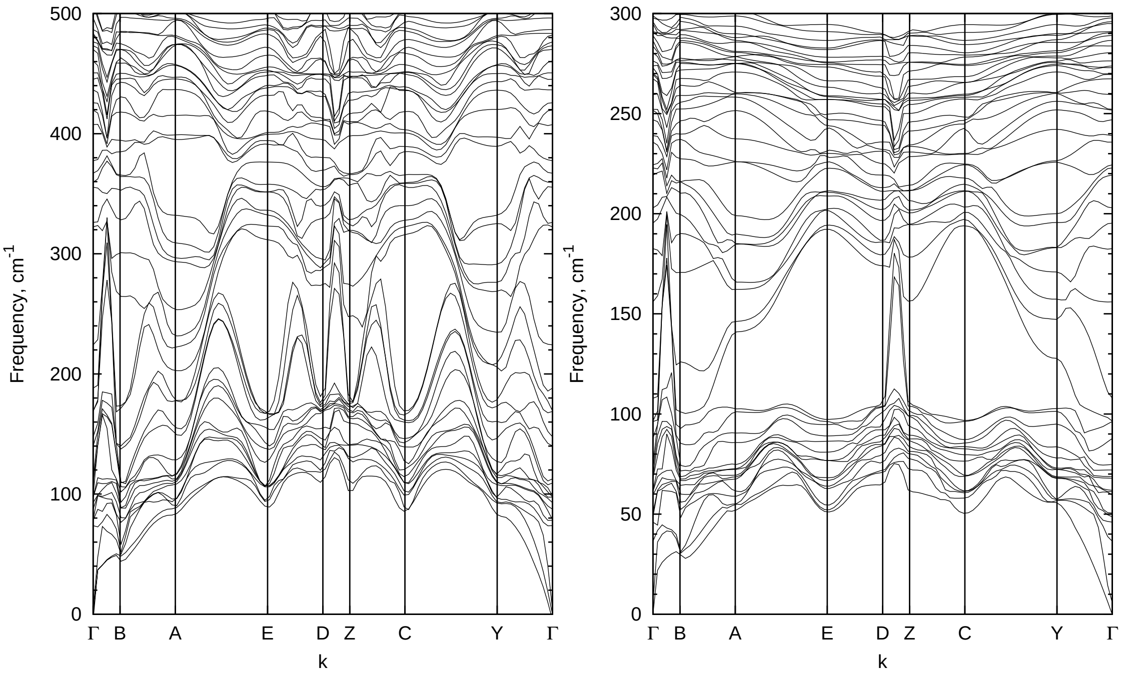


FIG. 1: Phonon bands for #26 silicon and germanium structures.

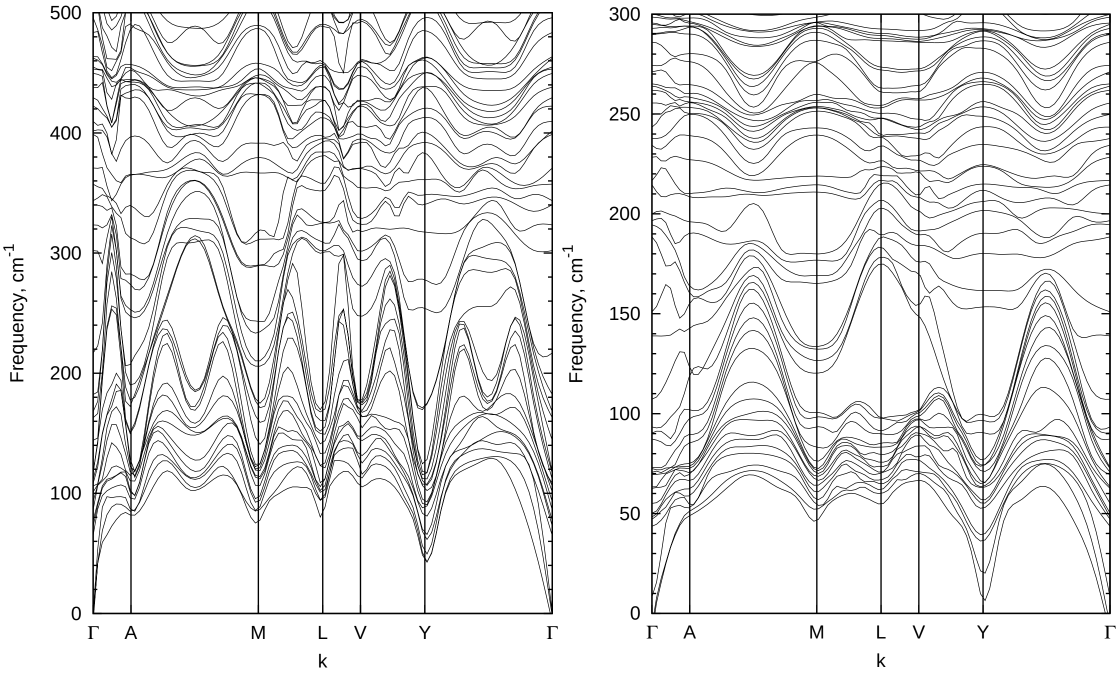


FIG. 2: Phonon bands for #27 silicon and germanium structures.

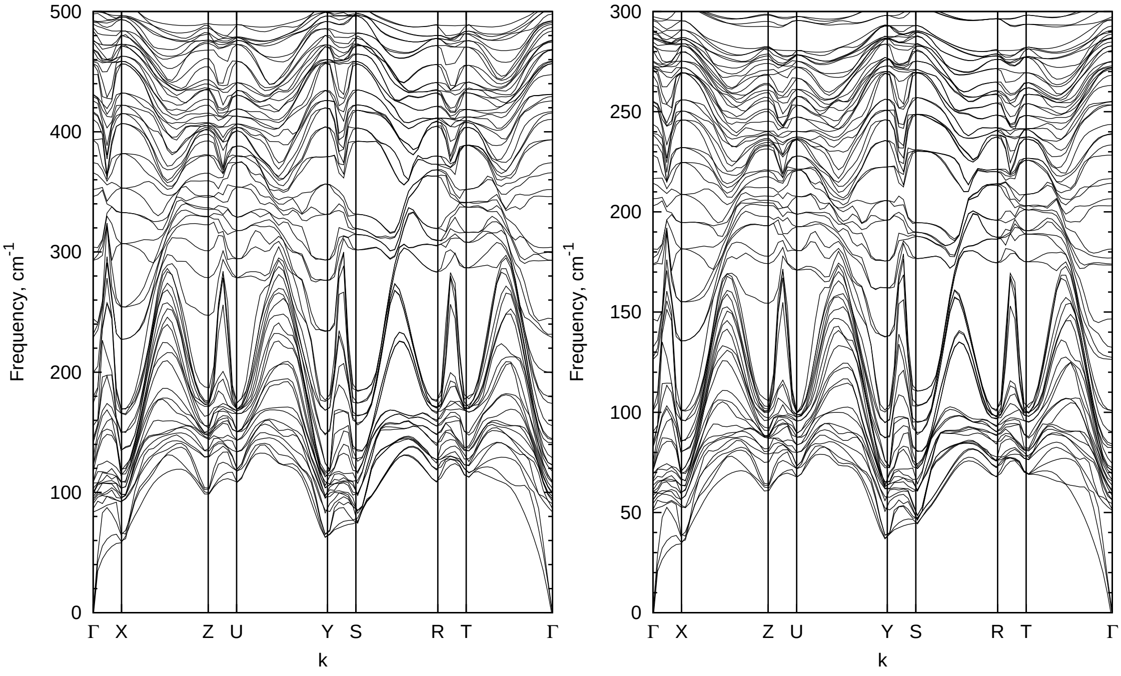


FIG. 3: Phonon bands for #28 silicon and germanium structures.

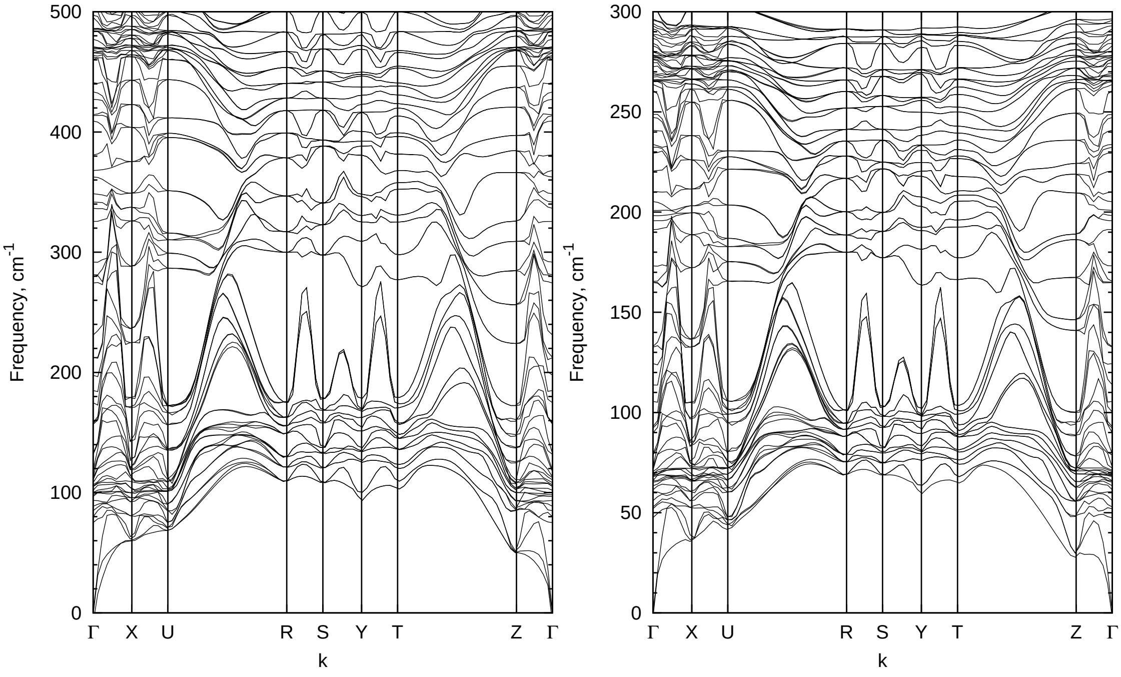


FIG. 4: Phonon bands for #50 silicon and germanium structures.

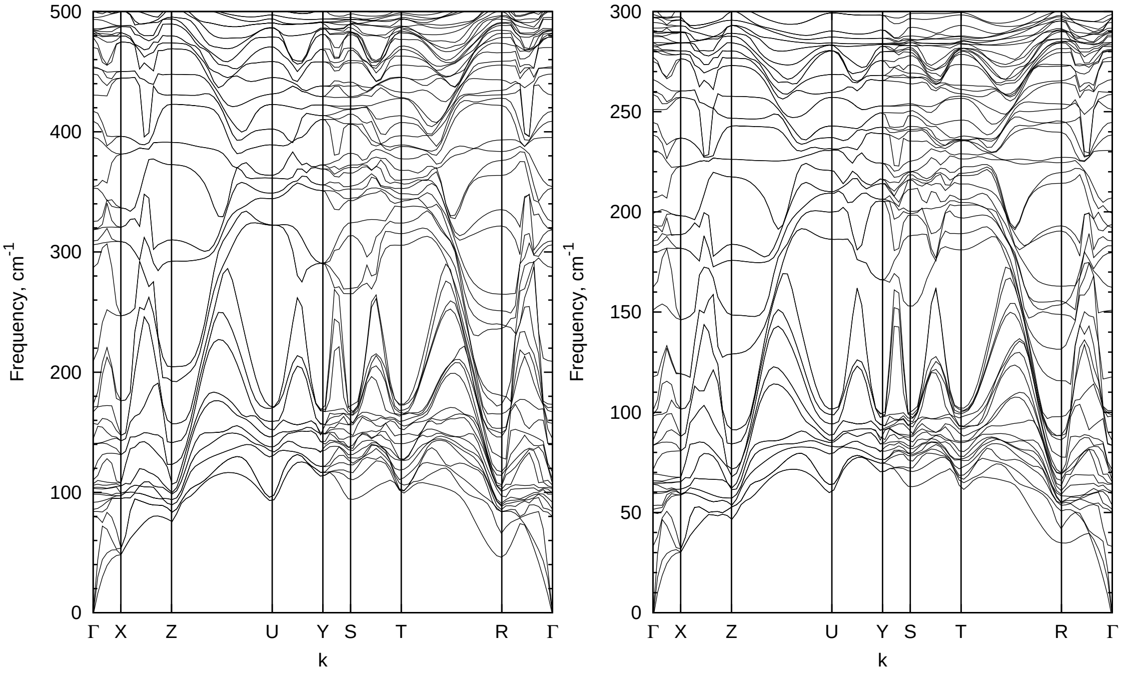


FIG. 5: Phonon bands for #55 silicon and germanium structures.

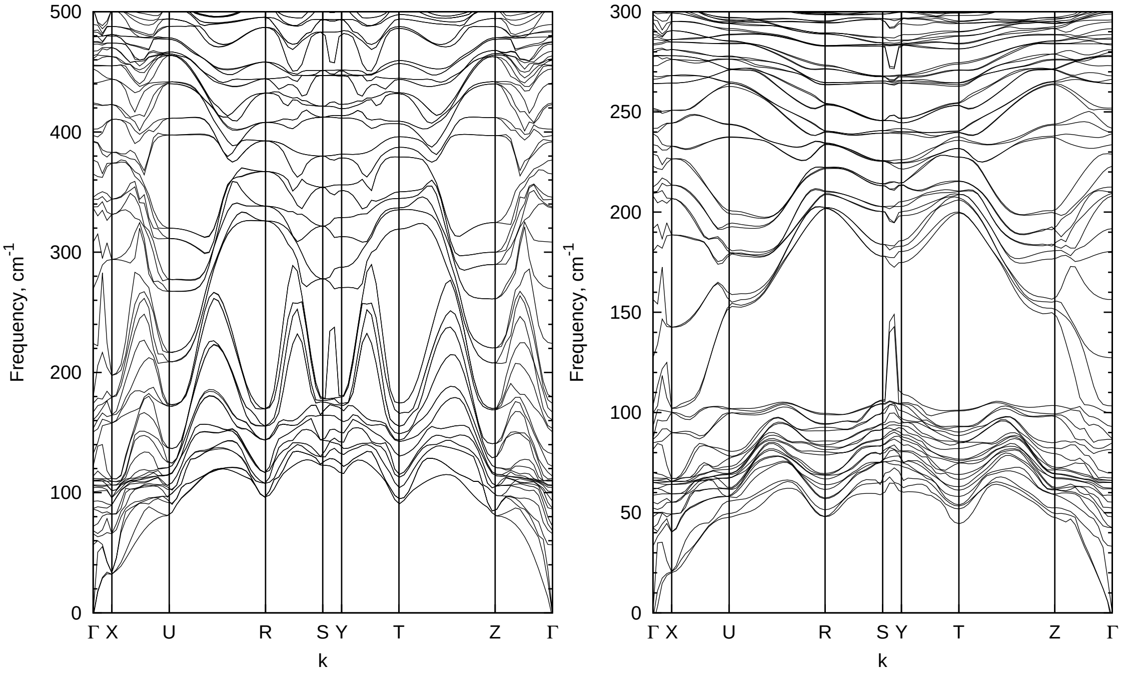


FIG. 6: Phonon bands for #88 silicon and germanium structures.

### E. Raman shift spectra for silicon and germanium allotropes

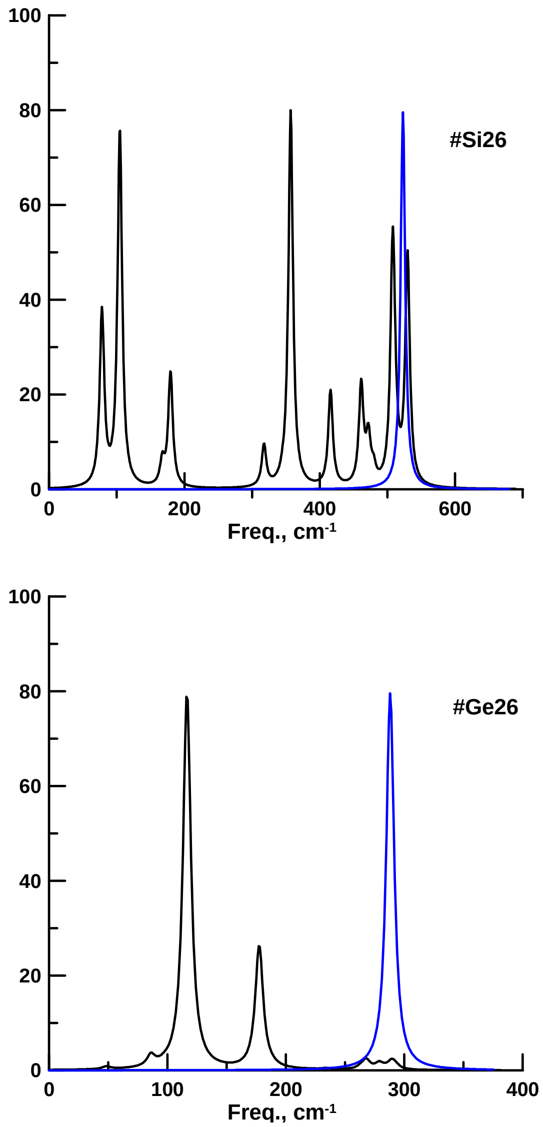


FIG. 7: Raman shift spectra for #26 (black lines) and diamond (blue lines) silicon (top panel) and germanium (bottom panel) structures.

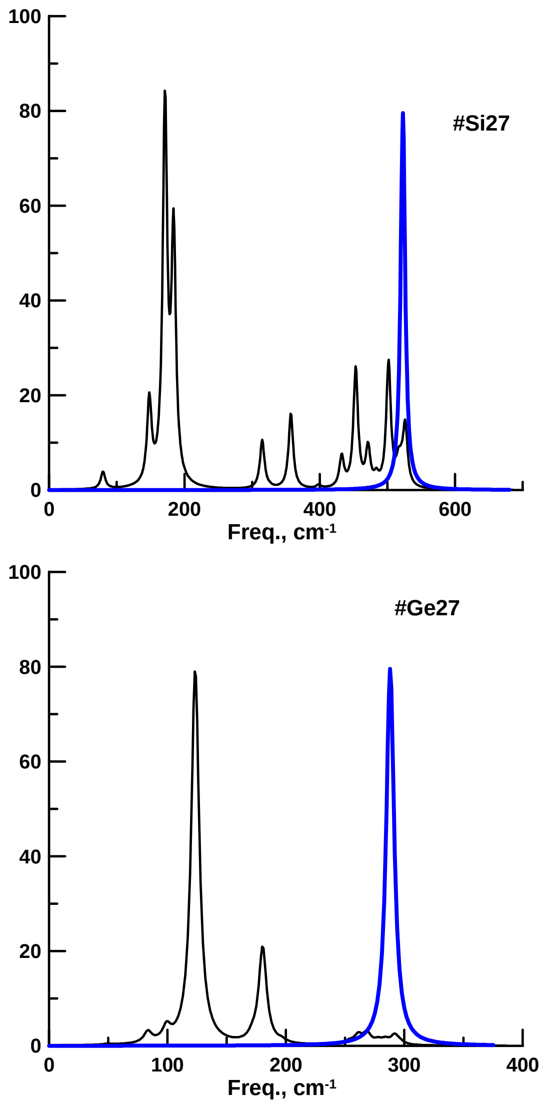


FIG. 8: Raman shift spectra for #27 (black lines) and diamond (blue lines) silicon (top panel) and germanium (bottom panel) structures.

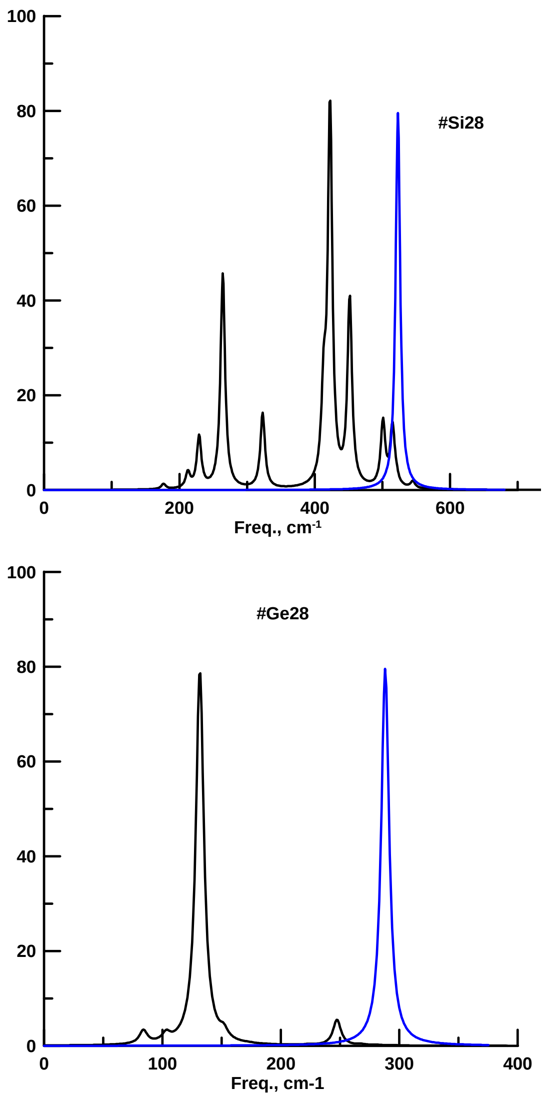


FIG. 9: Raman shift spectra for #28 (black lines) and diamond (blue lines) silicon (top panel) and germanium (bottom panel) structures.

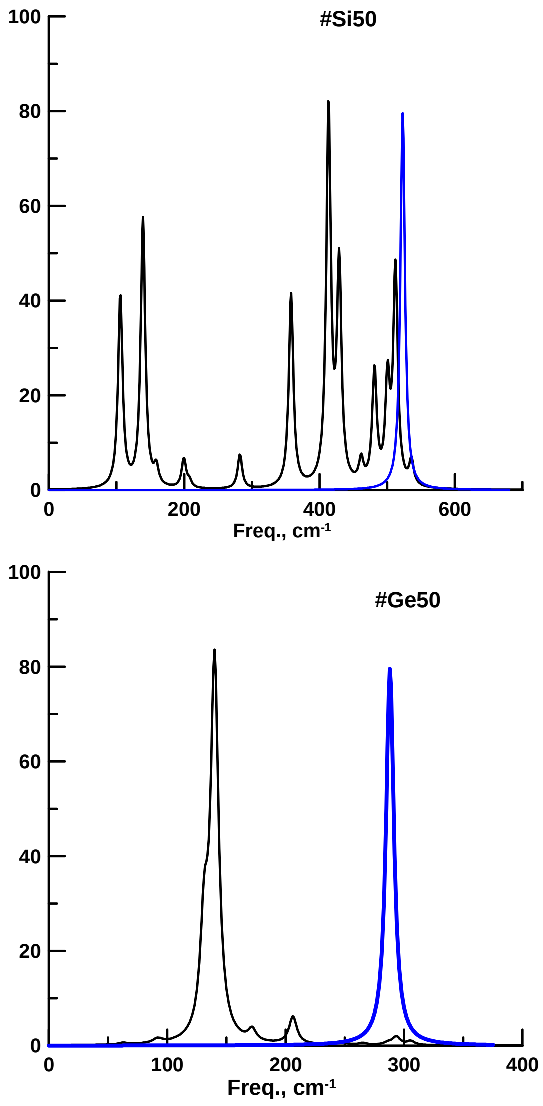


FIG. 10: Raman shift spectra for #50 (black lines) and diamond (blue lines) silicon (top panel) and germanium (bottom panel) structures.

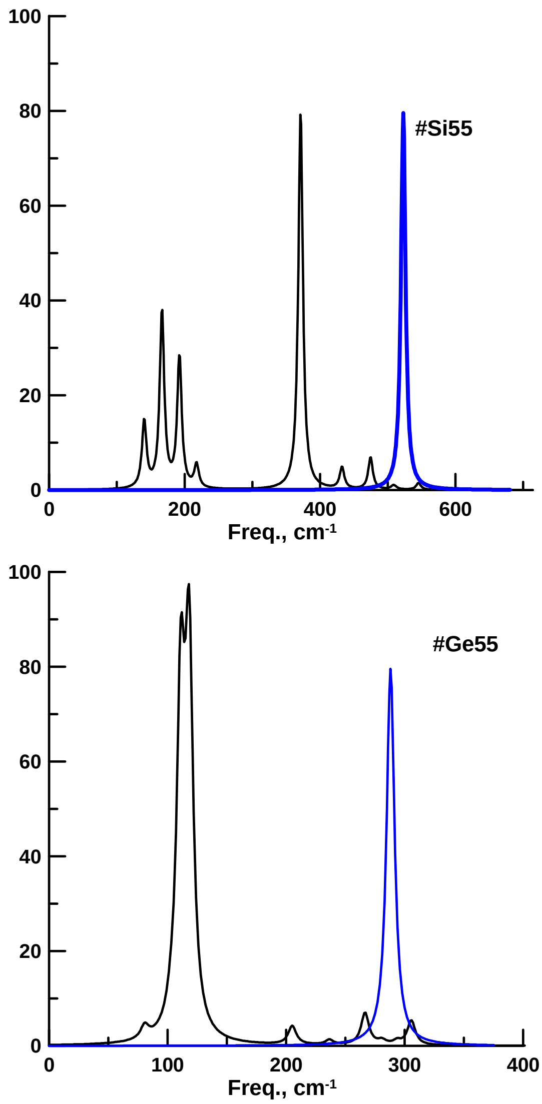


FIG. 11: Raman shift spectra for #55 (black lines) and diamond (blue lines) silicon (top panel) and germanium (bottom panel) structures.

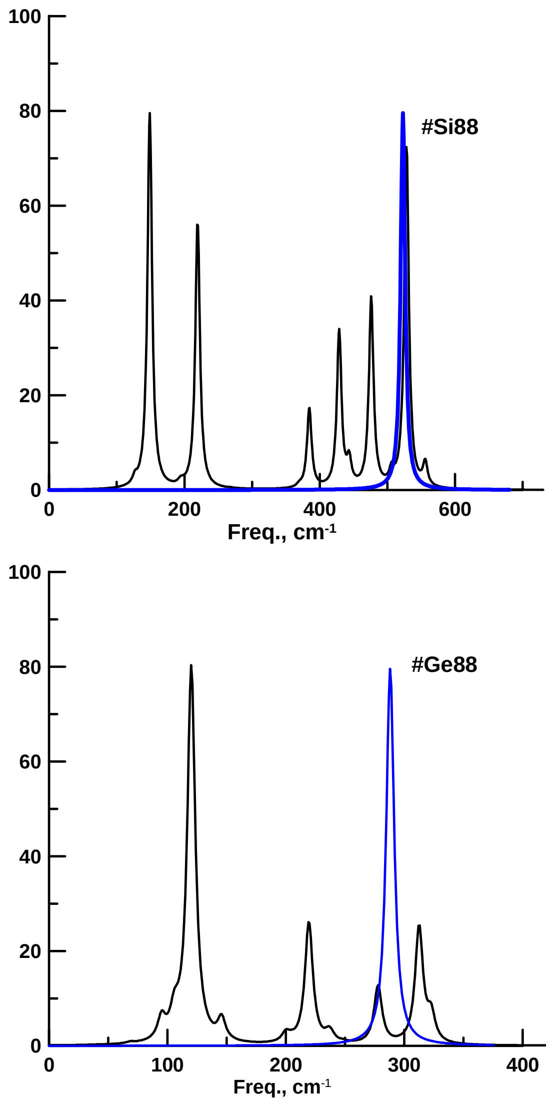


FIG. 12: Raman shift spectra for #88 (black lines) and diamond (blue lines) silicon (top panel) and germanium (bottom panel) structures.

### F. IR absorbtion spectra for silicon and germanium allotropes

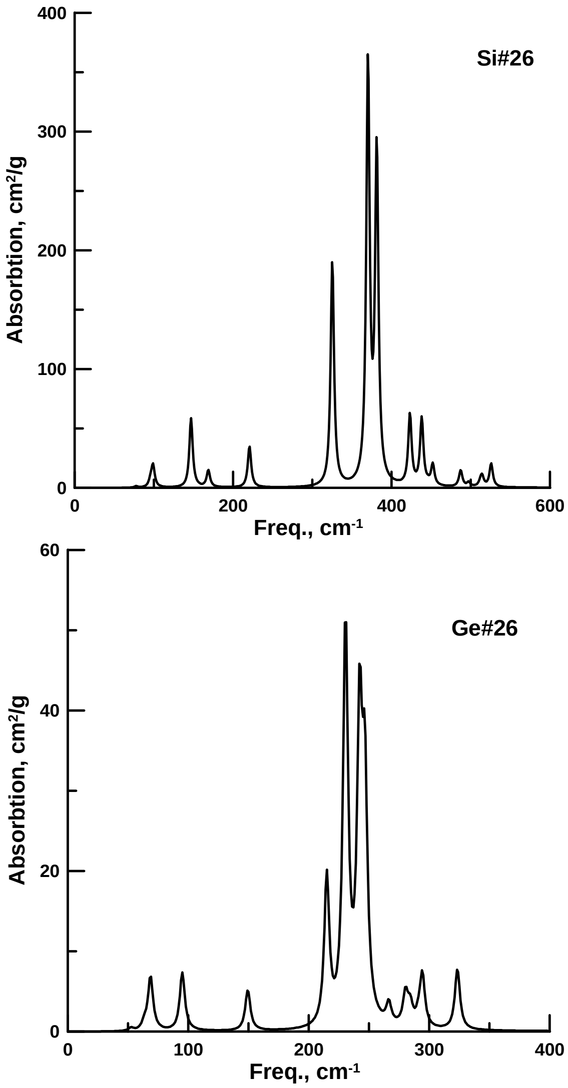


FIG. 13: IR absorbtion spectra for #26 silicon (top panel) and germanium (bottom panel) structures.

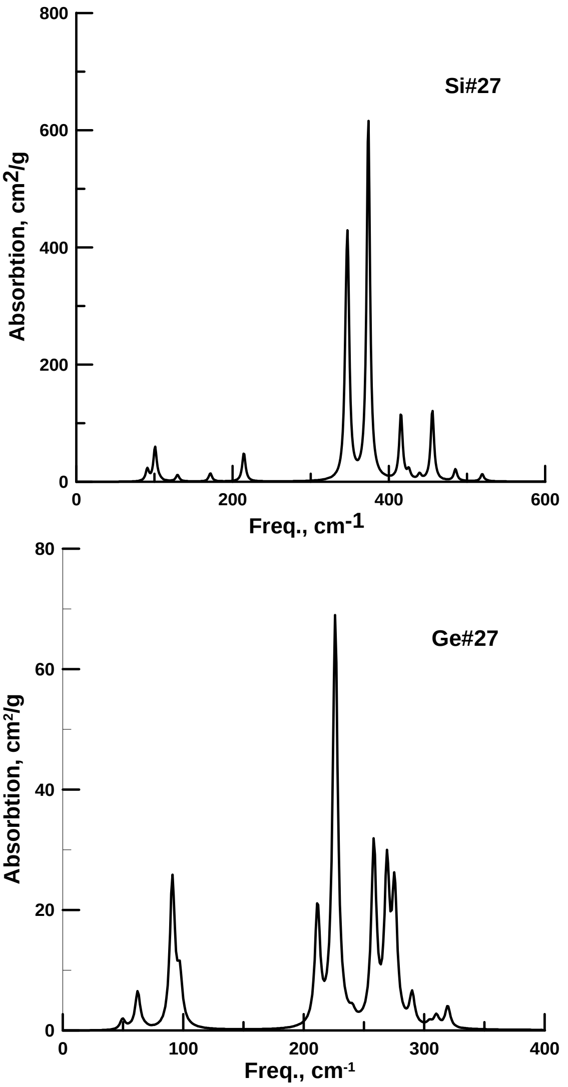


FIG. 14: IR absorbtion spectra for #27 silicon (top panel) and germanium (bottom panel) structures.

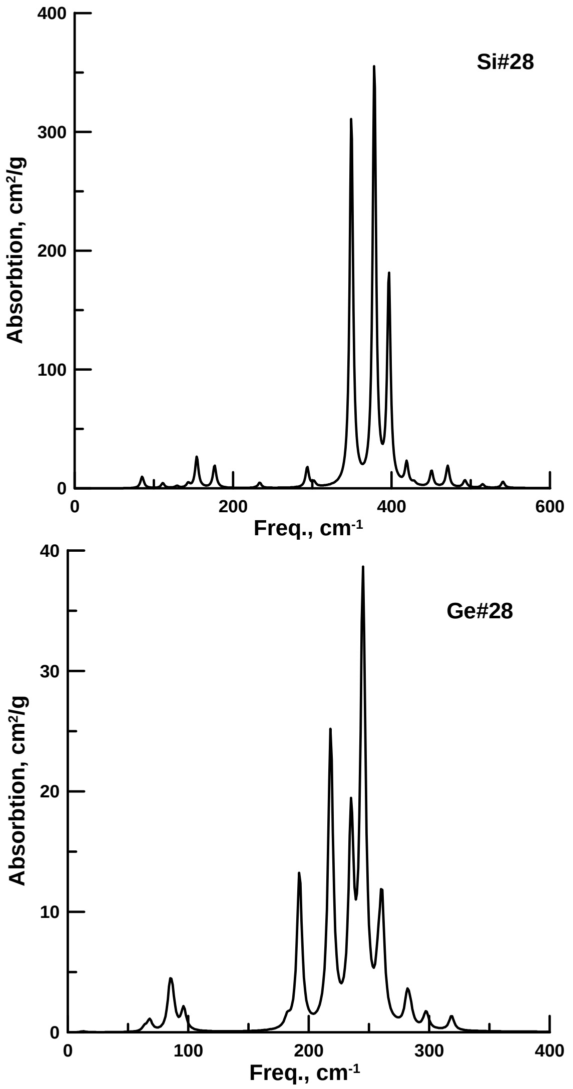


FIG. 15: IR absorbtion spectra for #28 silicon (top panel) and germanium (bottom panel) structures.

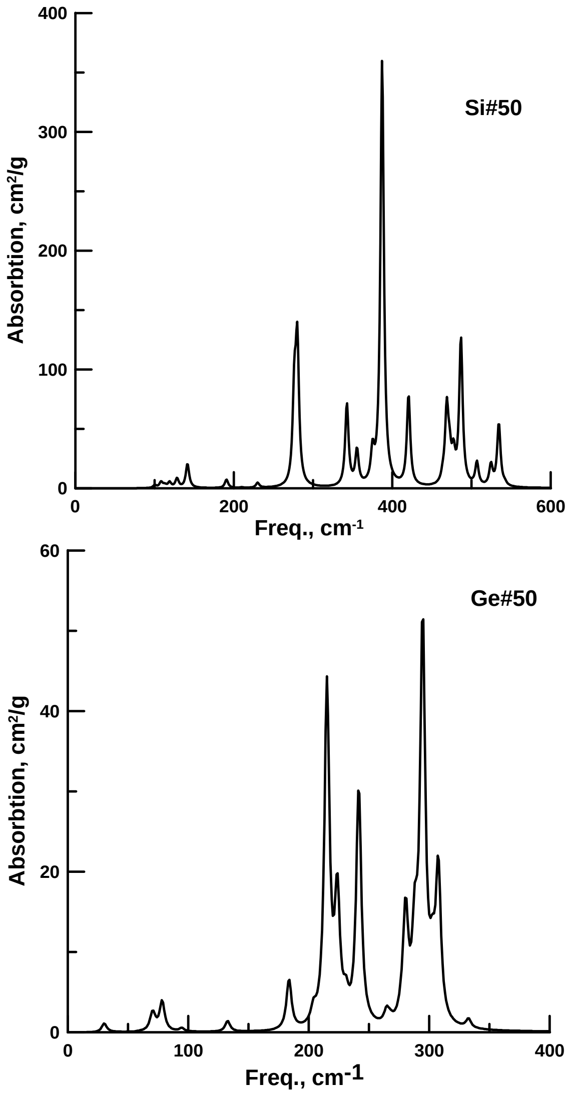


FIG. 16: IR absorbtion spectra for #50 silicon (top panel) and germanium (bottom panel) structures.

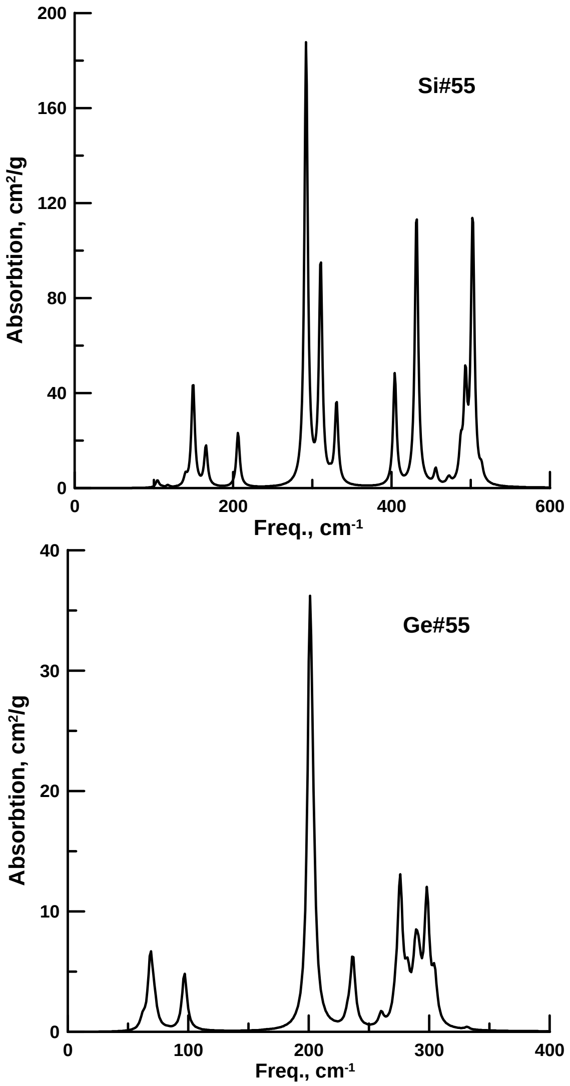


FIG. 17: IR absorbtion spectra for #55 silicon (top panel) and germanium (bottom panel) structures.

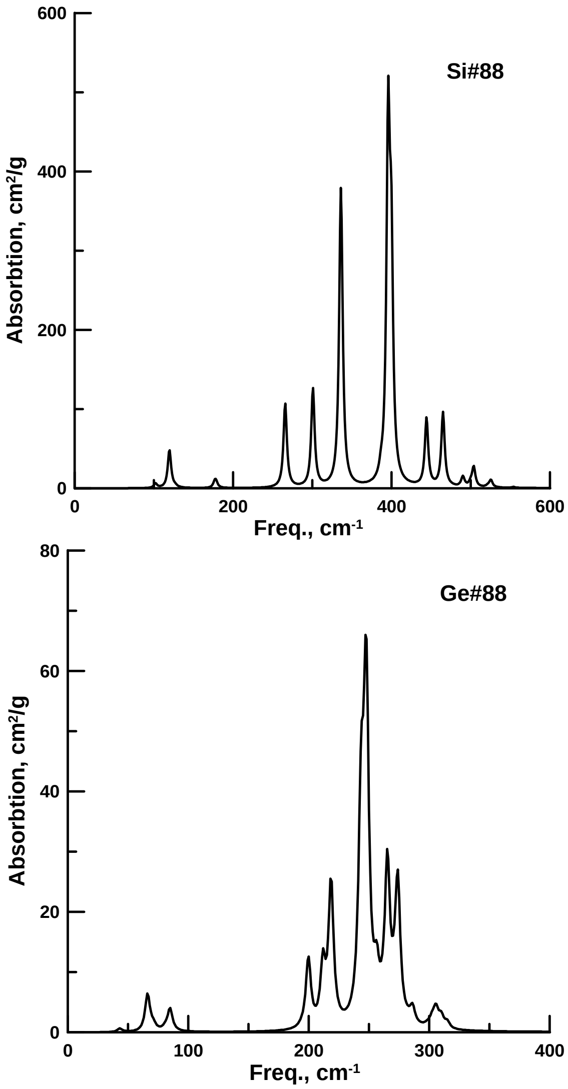


FIG. 18: IR absorbtion spectra for #88 silicon (top panel) and germanium (bottom panel) structures.

## G. Electronic bands and DOS for silicon and germanium allotropes

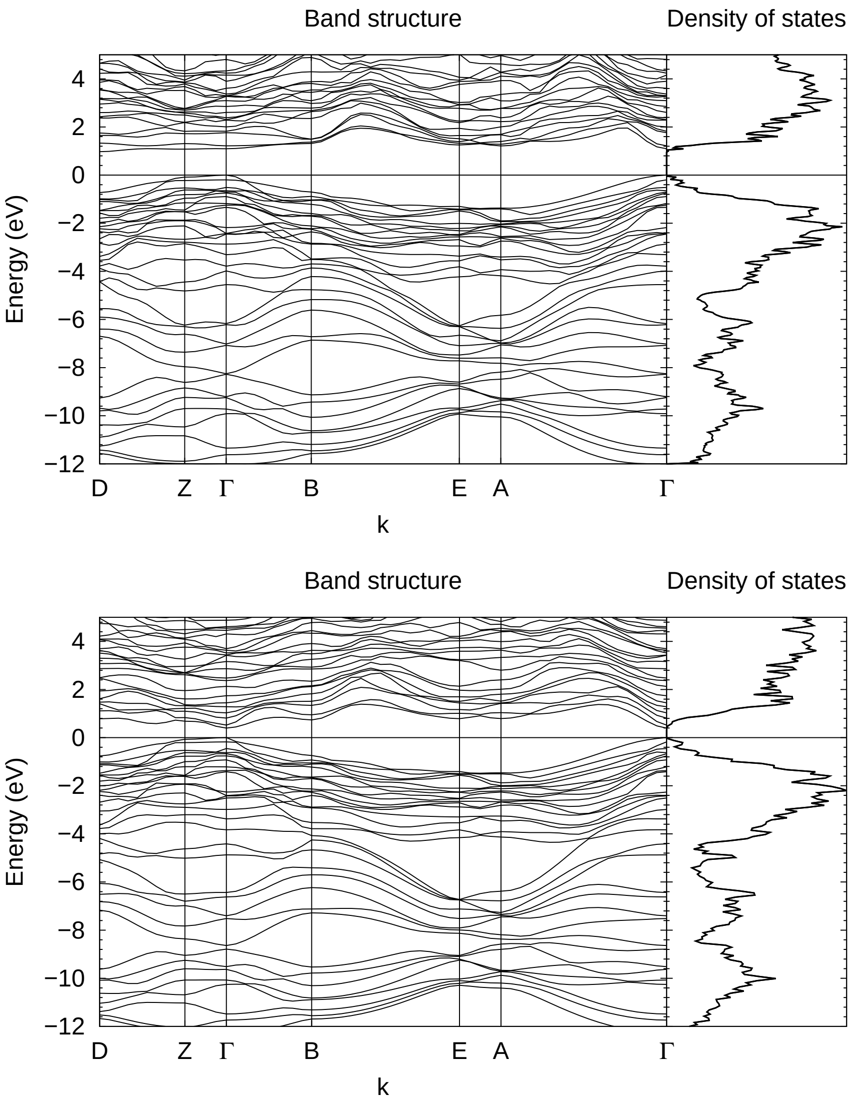


FIG. 19: Electronic bands and DOS for #26 silicon (top panel) and germanium (bottom panel) structures.

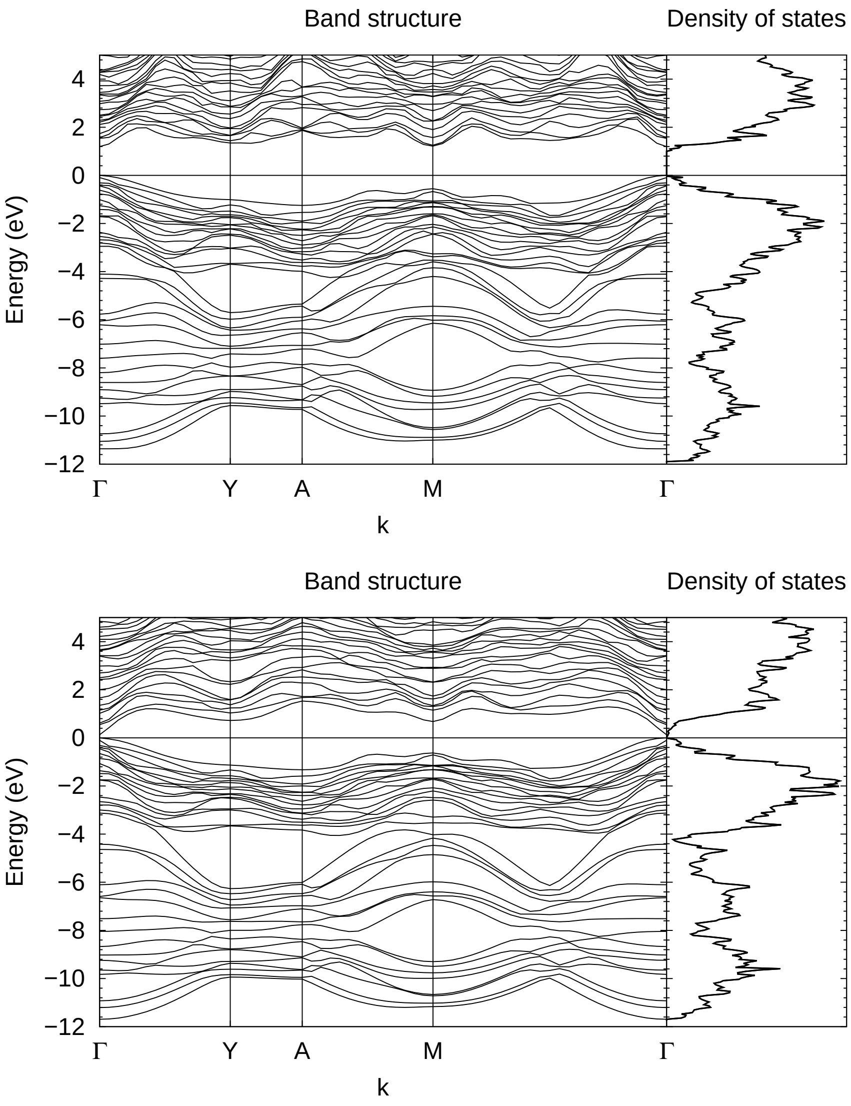


FIG. 20: Electronic bands and DOS for #27 silicon (top panel) and germanium (bottom panel) structures.

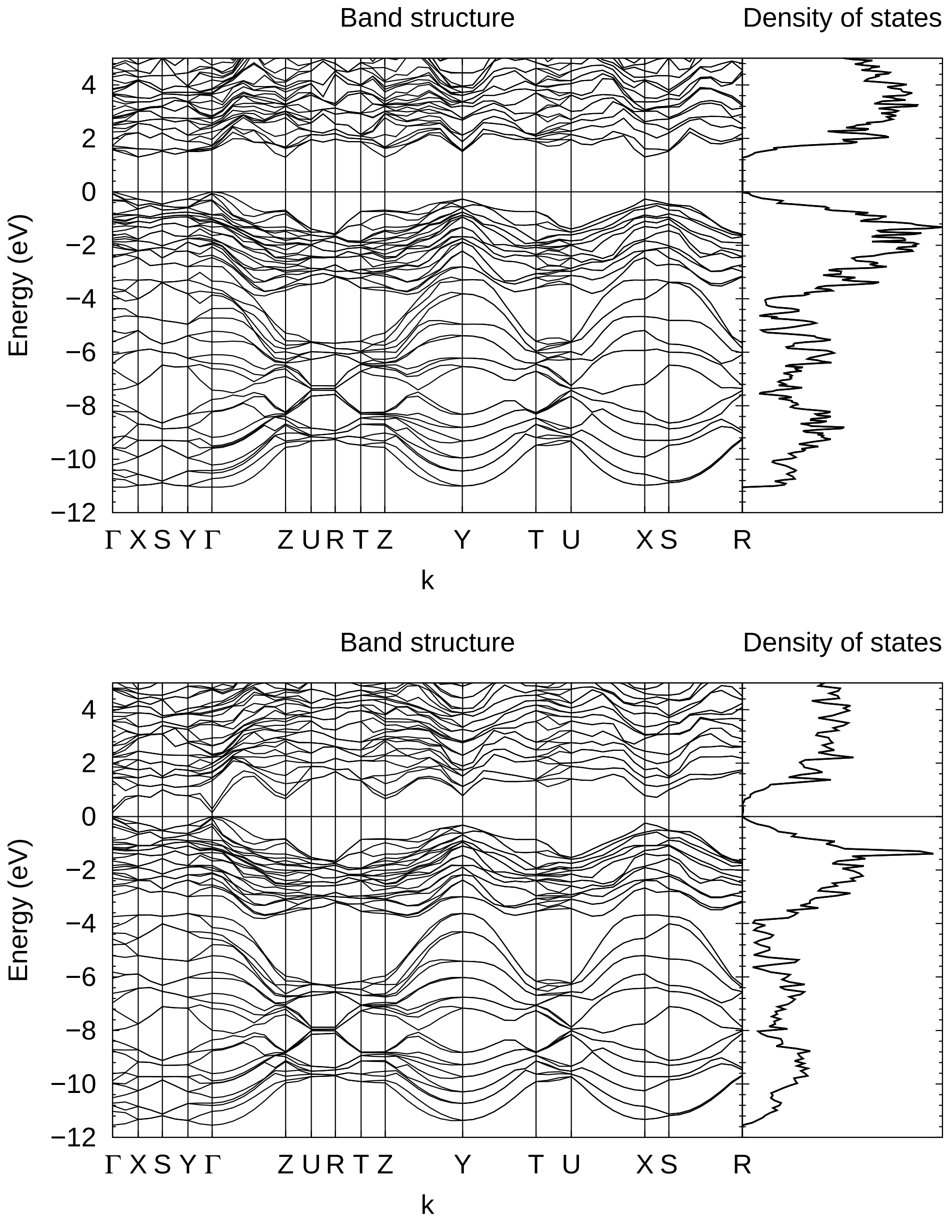


FIG. 21: Electronic bands and DOS for #28 silicon (top panel) and germanium (bottom panel) structures.

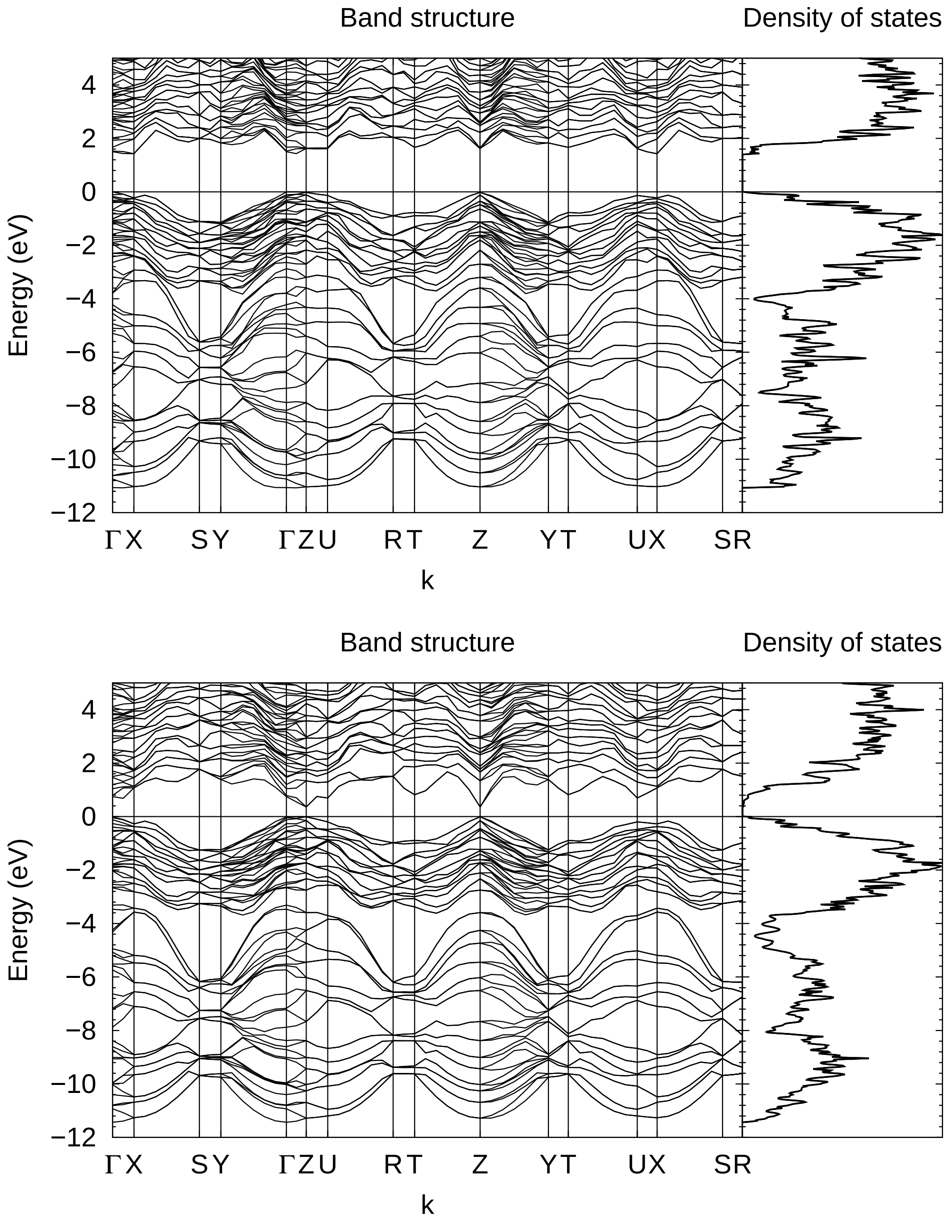


FIG. 22: Electronic bands and DOS for #50 silicon (top panel) and germanium (bottom panel) structures.

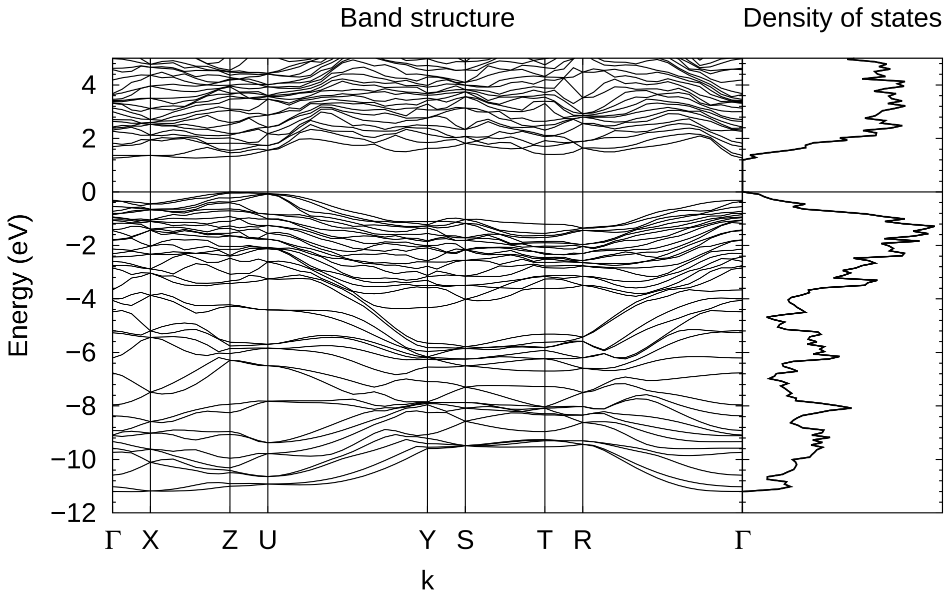


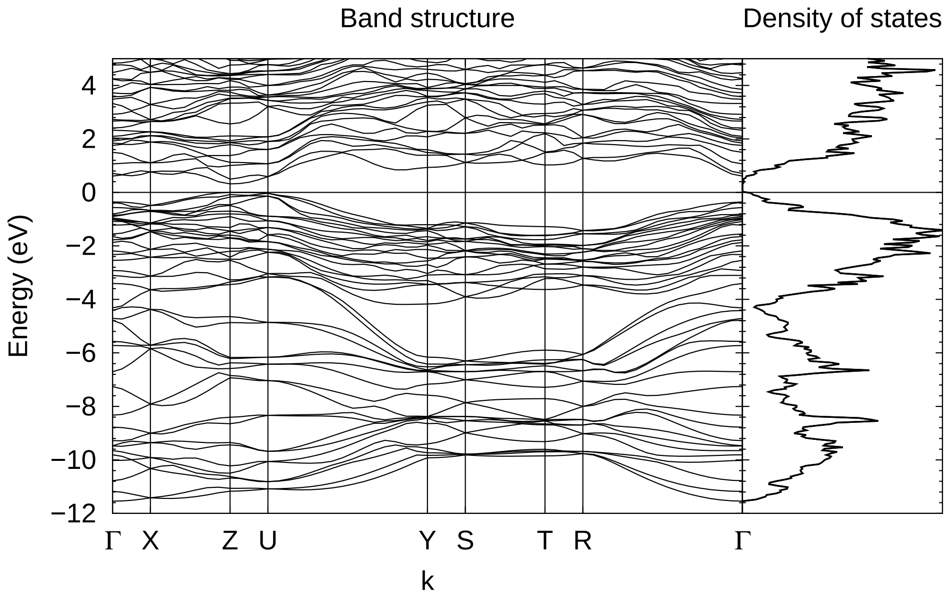


FIG. 23: Electronic bands and DOS for #55 silicon (top panel) and germanium (bottom panel) structures.

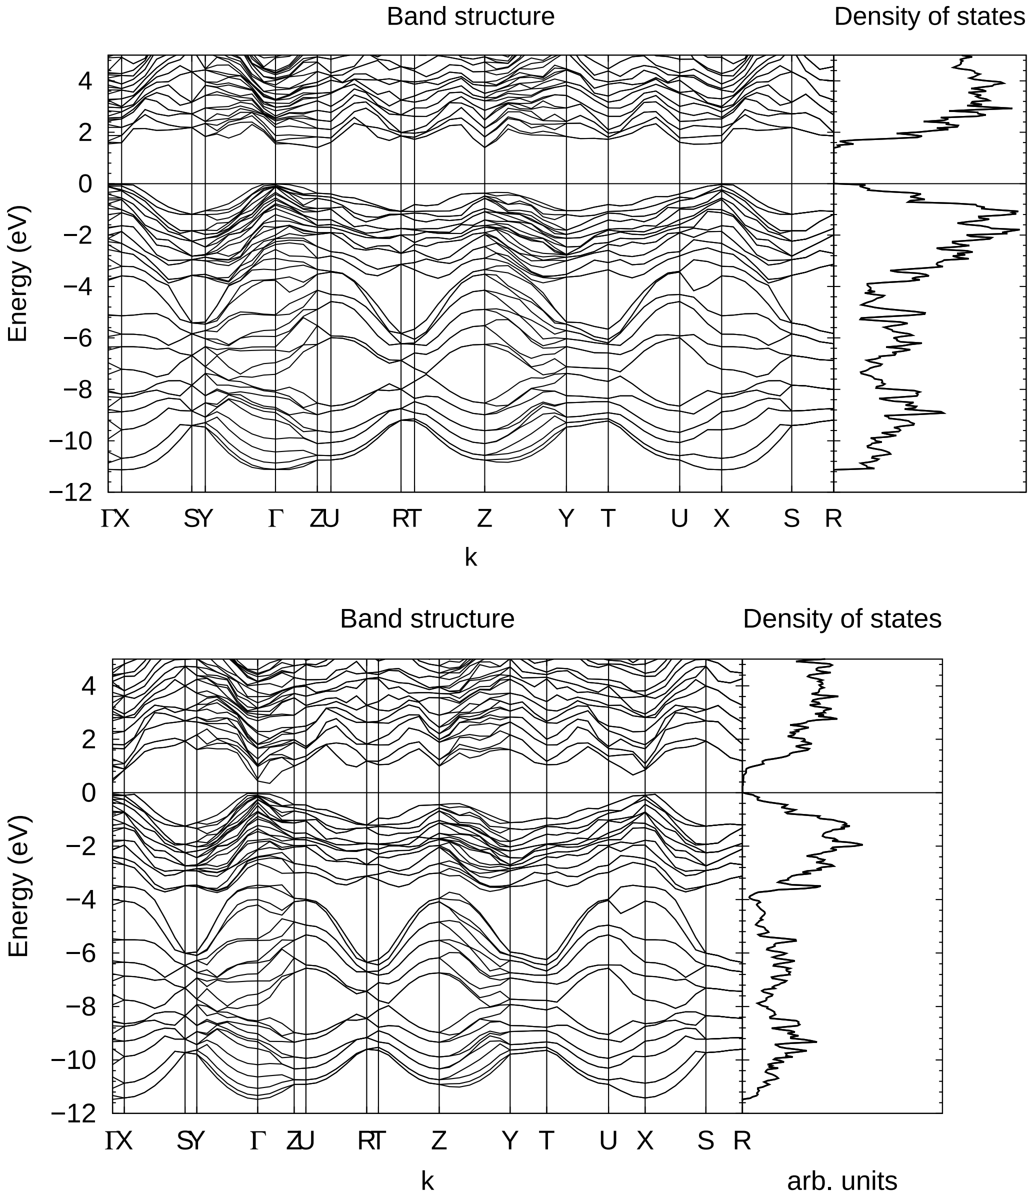


FIG. 24: Electronic bands and DOS for #88 silicon (top panel) and germanium (bottom panel) structures.
